# Supplementary material for: Deep Generative Data Assimilation in Multimodal Setting
Source: arXiv:2404.06665 source file (2024-06-12)
Supplement: Supplementary file 1 [file X_suppl.tex]

\clearpage
\setcounter{page}{1}
\setcounter{section}{0}
\setcounter{equation}{0}
\maketitlesupplementary
